# Supplementary material for: ICSFuzz: Collision Detector Bug Discovery in Autonomous Driving Simulators
Source: arXiv:2408.05694 source file (2024-08-11)
Supplement: Supplementary file 1 [file z_appendix.tex]

\newpage 

\appendix

% \huang{The lists of xxx are not needed}

%%
% \section{Ablation Study of Control Factors}
% \label{sec:appdenix:1}

% \listoftables

%%
\section{Evaluation of Multiple Control Factors Correlation}
\label{sec:eval:multiple_factor}

%%  Relationship 1: Speed vs Distance
%%
\begin{figure}[tp]
  \centering
  \begin{subfigure}[t]{0.23\textwidth}
    \includegraphics[width=\textwidth]{fig/result/multi_feature_distance-with-speed/SR-speed-distance-bar-FLB.png}
    \caption{Follow Leading Bicycle}
    \label{fig:sr-distance-speed_flb}
  \end{subfigure}
  \hfill
  \begin{subfigure}[t]{0.23\textwidth}
    \includegraphics[width=\textwidth]{fig/result/multi_feature_distance-with-speed/SR-speed-distance-bar-FLV.png}
    \caption{Follow Leading Vehicle}
    \label{fig:sr-distance-speed_flv}
  \end{subfigure}

  % \vspace{1em}
  \begin{subfigure}[t]{0.23\textwidth}
    \includegraphics[width=\textwidth]{fig/result/multi_feature_distance-with-speed/SR-speed-distance-bar-PSF.png}
    \caption{Pedestrian Standing Front}
    \label{fig:sr-distance-speed_psf}
  \end{subfigure}
  \hfill
  \begin{subfigure}[t]{0.23\textwidth}
    \includegraphics[width=\textwidth]{fig/result/multi_feature_distance-with-speed/SR-speed-distance-bar-LC.png}
    \caption{LaneChange}
    \label{fig:sr-distance-speed_lc}
  \end{subfigure}

  % \vspace{1em}
  \begin{subfigure}[t]{0.23\textwidth}
    \includegraphics[width=\textwidth]{fig/result/multi_feature_distance-with-speed/SR-speed-distance-bar-PCF.png}
    \caption{Pedestrian Crossing Front}
    \label{fig:sr-distance-speed_pcf}
  \end{subfigure}
  \hfill
  \begin{subfigure}[t]{0.23\textwidth}
    \includegraphics[width=\textwidth]{fig/result/multi_feature_distance-with-speed/SR-speed-distance-bar-InC.png}
    \caption{Intersection Collision}
    \label{fig:sr-distance-speed_inc}
  \end{subfigure}
  \caption{\S~\ref{sec:eval:multiple_factor}: Relationship between ICS SR and Collision Distance at Different Collision Speed Scope.}
  \label{fig:IC_SR-distance-speed}
\end{figure}

\textbf{Q1. Does the search direction for collision speed change at different collision distances?}
% no, collision speed still doesn't have a large impact compared with collision distance

From Figure~\ref{fig:IC_SR-distance-speed}, when examining three specific collision distance groups, the trend for three different collision speed groups remains relatively consistent compared to not considering the collision distance.
% it can be observed that for three specific collision distance groups, there is not a significant variation across different collision speed ranges.
% The trend confirms the conclusion drawn in \S~\ref{eval:rq3-single_feature} regarding the limited impact of collision speed as a single feature, indicating that collision speed does not significantly contribute to the search for IC events.

%%  Relationship 1:  Distance with speed

%%
\begin{figure}[tp]
  \centering
  \begin{subfigure}[t]{0.23\textwidth}
    \includegraphics[width=\textwidth]{fig/result/multi_feature_speed-with-distance/SR-distance-speed-FLB.png}
    \caption{Follow Leading Bicycle}
    \label{fig:sr-distance_speed_flb}
  \end{subfigure}
  \hfill
  \begin{subfigure}[t]{0.23\textwidth}
    \includegraphics[width=\textwidth]{fig/result/multi_feature_speed-with-distance/SR-distance-speed-FLV.png}
    \caption{Follow Leading Vehicle}
    \label{fig:sr-distance_speed_flv}
  \end{subfigure}

  \vspace{1em}
  \begin{subfigure}[t]{0.23\textwidth}
    \includegraphics[width=\textwidth]{fig/result/multi_feature_speed-with-distance/SR-distance-speed-PSF.png}
    \caption{Pedestrian Standing Front}
    \label{fig:sr-distance_speed_psf}
  \end{subfigure}
  \hfill
  \begin{subfigure}[t]{0.23\textwidth}
    \includegraphics[width=\textwidth]{fig/result/multi_feature_speed-with-distance/SR-distance-speed-LC.png}
    \caption{Lane Change}
    \label{fig:sr-distance_speed_lc}
  \end{subfigure}

  \vspace{1em}
  \begin{subfigure}[t]{0.23\textwidth}
    \includegraphics[width=\textwidth]{fig/result/multi_feature_speed-with-distance/SR-distance-speed-PCF.png}
    \caption{Pedestrian Crossing Front}
    \label{fig:sr-distance_speed_pcf}
  \end{subfigure}
  \hfill
  \begin{subfigure}[t]{0.231\textwidth}
    \includegraphics[width=\textwidth]{fig/result/multi_feature_speed-with-distance/SR-distance-speed-InC.png}
    \caption{Intersection Collision}
    \label{sec:eval:multiple_factor}
  \end{subfigure}
\caption{\S~\ref{sec:eval:multiple_factor}: Relationship between ICS SR and Collision Speed at Different Collision Distance Scope.}
\label{fig:IC_SR-speed-distance}
\end{figure}

\textbf{Q2. Does the search direction for collision distance change at different collision speed scopes?}
Figure~\ref{fig:IC_SR-speed-distance} shows the trends in the SR across different collision distances for three collision speed scopes.
The observed patterns strongly support the conclusion made in \S~\ref{sec:eval:rq3_search_direction} regarding the impact of collision distance as a single feature.
In most scenarios, a high collision speed consistently results in more ICSs when combined with a far collision distance.
Except for PCF, a combination of close collision distance and high collision speed leads to more identified ICSs. 

% the effective search direction indicates increased collision distance.
% For PSF, the effective search direction suggests a decrease in collision distance.

%% Relationship 2: Angle vs Speed 
\begin{figure}[tp]
  \centering
  \begin{subfigure}[t]{0.22\textwidth}
    \includegraphics[width=\textwidth]{fig/result/multi_feature_speed-angle/SR-speed-angle-line-FLB.png}
    \caption{Follow Leading Bicycle}
    \label{fig:sr-speed-angle-flb}
  \end{subfigure}
  \hfill
  \begin{subfigure}[t]{0.22\textwidth}
    \includegraphics[width=\textwidth]{fig/result/multi_feature_speed-angle/SR-speed-angle-line-FLV.png}
    \caption{Follow Leading Vehicle}
    \label{fig:sr-speed-angle-flv}
  \end{subfigure}

  % \vspace{1em}

  \begin{subfigure}[t]{0.22\textwidth}
    \includegraphics[width=\textwidth]{fig/result/multi_feature_speed-angle/SR-speed-angle-line-LC.png}
    \caption{Lane Change}
    \label{fig:sr-speed-angle-lc}
  \end{subfigure}
  \hfill
  \begin{subfigure}[t]{0.22\textwidth}
    \includegraphics[width=\textwidth]{fig/result/multi_feature_speed-angle/SR-speed-angle-line-PSF.png}
    \caption{Pedestrian Standing Front}
    \label{fig:sr-speed-angle-psf}
  \end{subfigure}

  % \vspace{1em}

  \begin{subfigure}[t]{0.22\textwidth}
    \includegraphics[width=\textwidth]{fig/result/multi_feature_speed-angle/SR-speed-angle-line-PCF.png}
    \caption{Pedestrian Crossing Front}
    \label{fig:sr-speed-angle-pcf}
  \end{subfigure}
  \hfill
  \begin{subfigure}[t]{0.22\textwidth}
    \includegraphics[width=\textwidth]{fig/result/multi_feature_speed-angle/SR-speed-angle-line-InC.png}
    \caption{Intersection Collision}
    \label{fig:sr-speed-angle-inc}
  \end{subfigure}
\caption{\S~\ref{sec:eval:multiple_factor}: Relationship between ICS SR and Collision Angle at Different Collision Speed Scope.}
  \label{fig:IC_SR-speed-angle}
\end{figure}

\textbf{Q3. Does the search direction for collision angle change at different collision speed scopes?}
The relationship between ICS occurrences and the collision angle, as depicted in Figure~\ref{fig:IC_SR-speed-angle}, remains largely unchanged across different collision speed conditions compared to the trend without considering the effect of collision speed shown in Figure~\ref{fig:IC_SR-angle}.
The effective search directions for the collision angle remain consistent across different speed scopes, similar to when considering the collision angle independently. 
In scenario InC, a distinct data trend difference at low collision speed is observed at positive collision angles.
However, since the pattern is not observed in other scenarios, it is likely attributed to data noise.
% The relationship between SR and collision speed is still the same as shown in Figure~\ref{fig:IC_SR-speed}, even considering the collision angle.
% Th us, the data trend can be explained through similar reasons.
% The observed trends and search directions mentioned above indicate that collision speed does not affect the collision angle either, which further confirms that collision speed does not play a significant role.

%% Relationship 3: Distance vs Speed.
%%
\begin{figure}[tp]
  \centering
  \begin{subfigure}[t]{0.22\textwidth}
    \includegraphics[width=\textwidth]{fig/result/multi_feature_distance-angle/SR-distance-angle-FLB.png}
    \caption{Follow Leading Bicycle}
    \label{fig:sr-dist-angle-flb}
  \end{subfigure}
  \hfill
  \begin{subfigure}[t]{0.22\textwidth}
    \includegraphics[width=\textwidth]{fig/result/multi_feature_distance-angle/SR-distance-angle-FLV.png}
    \caption{Follow Leading Vehicle}
    \label{fig:sr-dist-angle-flv}
  \end{subfigure}
  % \vspace{1em}
  \begin{subfigure}[t]{0.22\textwidth}
    \includegraphics[width=\textwidth]{fig/result/multi_feature_distance-angle/SR-distance-angle-LC.png}
    \caption{Lane Change}
    \label{fig:sr-dist-angle-lc}
  \end{subfigure}
  \hfill
  \begin{subfigure}[t]{0.22\textwidth}
    \includegraphics[width=\textwidth]{fig/result/multi_feature_distance-angle/SR-distance-angle-PSF.png}
    \caption{Pedestrian Standing Front}
    \label{fig:sr-dist-angle-psf}
  \end{subfigure}
  % \vspace{1em}
  \begin{subfigure}[t]{0.22\textwidth}
    \includegraphics[width=\textwidth]{fig/result/multi_feature_distance-angle/SR-distance-angle-PCF.png}
    \caption{Pedestrian Crossing Front}
    \label{fig:sr-dist-angle-pcf}
  \end{subfigure}
  \hfill
  \begin{subfigure}[t]{0.22\textwidth}
    \includegraphics[width=\textwidth]{fig/result/multi_feature_distance-angle/SR-distance-angle-InC.png}
    \caption{Intersection Collision}
    \label{fig:sr-dist-angle-inc}
  \end{subfigure}

  \caption{\S~\ref{sec:eval:multiple_factor}: Relationship between ICS SR and Collision Angle at Different Distance.}
  \label{fig:IC_SR-dist-angle}
\end{figure}

% \textbf{Q4. Can \sysname precisely identify all IC events?} 
\textbf{Q4. Does the search direction for collision angle change at different collision distance scopes?} 

When considering the variations of collision angle across different collision distances, the observed data trend differs slightly from considering collision angle alone in Figure~\ref{fig:IC_SR-angle}.
In scenarios LC, PSF, and InC, the data aligns with the trend of increasing collision angle, bringing more ICSs.
Similarly, although there are fewer fluctuations in the middle collision distance scope in scenario FLV, the overall trend still holds. 
Moreover, the SR exhibits a higher slope at greater collision distances, indicating that simultaneously increasing both collision distance and collision angle can lead to more ICSs.

In this scenario FLB(see Figure~\ref{fig:sr-dist-angle-flb}), the relationship between collision angle and final SR is unstable and exhibits significant fluctuations under far collision distances. 
% The effective search direction for collision angle is increasing the angle to the positive direction at low collision distances.
% For middle and far collision distances, the search direction, searching from the middle toward both ends.
For collision in middle and far distances, the trend similar to the total trend in general. 
But the middle collision distance brings more ICS.
When considering the collision distance and collision angle together, the middle collision distance and the collision angle close to -1 and 1 create more ICSs.
% Changing driving behavior from a  collision distance can increase the likelihood of creating secondary collisions, which may explain the fluctuations in middle and far collision distances.

In scenario PCF, exceptions also occur at low collision distances. 
The exception results in different search directions for PCF at different collision distances compared to the one shown in Figure~\ref{fig:sr_angle-pcf}.
In the low collision distance scope, there are hardly any ICSs for the positive collision angle.
Hence, the search direction should be towards increasing negative collision angles.
Conversely, the situation is reversed in the middle and far collision distance scopes.
There are few collision incidents when the collision angle is negative, the search direction should be towards increasing to the positive collision angles.
The significant occurrence of ICSs in the negative collision angle zone at low collision distances can be attributed to the different relative positions between the EV and the NPC if changed driving behavior at different collision distances.

When driving behavior changes at low collision distances, the pedestrian just steps onto the lane, which corresponds to the negative collision angle region.
In order to collide with the pedestrians, the vehicle needs to veer towards the negative angle region.
On the other hand, at middle to high collision distances, the pedestrian has already reached the region marked by the positive collision angle by the time the EV approaches.
Hence, collision events are more likely to occur in this region.
Generally, collision scenarios with a moderate collision distance and collision angle close to 1, as well as collision scenarios with a low collision distance and negative collision angle, tend to result in a higher number of identified ICSs.

% our pre-defined search direction for collision distance.
% As for the collision angle, even though there may be fewer ICSs in certain conditions within the positive or negative collision angle ranges, our method of incrementally increasing the search direction from 0 in either positive or negative direction ensures we can still find a sufficient number of ICSs.

%% CrashFactors
%% 
\begin{table}[tp]
\centering
\caption{Collision Factors.}
%% resize the entire tabular
\resizebox{0.45\textwidth}{!}{
\begin{tabular}{|c|c|l|}
\toprule
%% header
\textbf{\makecell{Crash \\ Factors}}
& \textbf{Target}
& \textbf{Values}
\\
\hline
\midrule

%% factor: Time
\parbox[t]{0pt}{
\multirow{7}{*}{
    \rotatebox[origin=c]{90}{
        \textbf{Time}
    }
}
}
& \multirow{4}{*}[0pt]{AV}
& \makecell[l]{
    Daylight (43.75\%),
    Dark (56.25\%)
    ~\cite{divergent_effect}
} 
\\
\cline{3-3}
% -
& % -
& \makecell[l]{
    Daylight (67.3\%),   
    Unknown (32.7\%)
    ~\cite{avoid}
} 
\\
\cline{3-3}
% -
& % -
& \makecell[l]{
    Daylight (64.52\%), 
    Dark street lights (33.33\%),  
    \\
    Dusk-dawn (2.15\%)
    ~\cite{analysis_poi}
}
\\
\cline{3-3}
% -
& % -
& \makecell[l]{
    Daylight (45\%),     
    Other (43\%),   
    % \\
    Dark night (9\%),    
    Dusk-dawn (3\%)
    ~\cite{automated_latent}
} 
\\
\cline{2-3}
% -
& \multirow{3}{*}[5pt]{Bicycle}
& \makecell[l]{
    Good daytime lighting (46.4\%), 
    Poor daytime lighting (15.4\%),
    \\
    Poor lighting at night  (28.5\%),  
    Poor lighting at night (9.7\%)
    ~\cite{car-bicycle_analysis}
}
\\
\cline{3-3}
% -
& % - Bicycle
& \makecell[l]{  
    Daylight (52.2\%),
    Dark (30.1\%),
    Dusk or Dawn (17.8\%)
    ~\cite{single_bicycle_crash}
} 
\\
\cline{3-3}
% -
& % Bicycle
& \makecell[l]{
    Daytime (77.2\%),
    Nighttime w/ Lighting (18.3\%),
    \\
    Nighttime wo/ Lighting (4.5\%)
    ~\cite{identifying_factors}
} 
\\
\midrule
%% end Time

%% factor: collision type
\parbox[t]{4pt}{
\multirow{7}{*}[-50pt]{
    \rotatebox[origin=c]{90}{
        \textbf{\makecell{Collision Type}}
    }
}
}
& \multirow{6}{*}[-10pt]{AV}
& \makecell[l]{
    Rear-end: (59.38\%), 
    Other (40.63\%) 
    ~\cite{divergent_effect}
}
\\
\cline{3-3}
% -
& % AV
& \makecell[l]{
    Front (25.7\%),  
    Left (25.1\%),  
    Rear (21.2\%),
    Right (21\%),
    \\
    Top (4.5\%), 
    Bottom (2.4\%)
    ~\cite{avoid}
}  
\\
\cline{3-3}
% -
& % AV
& \makecell[l]{
    Rear-end (64\%), 
    Sideswipe (15\%), 
    Broadside (12\%),
    Head-on (12\%)
    ~\cite{analysis_poi}
}
\\
\cline{3-3}
% -
& % AV
& \makecell[l]{
    Rear-end (61.1\%),  
    Sideswipe (24.8\%), 
    Other (6.2\%), 
    \\
    Broadside (5.3\%), 
    Head-on (2.7\%)
    ~\cite{exploratory_cal}
} 
\\
\cline{3-3}
% -
& % AV
& \makecell[l]{
    Rear-end (49.85\%),  
    Sideswipe (20.64\%),
    Head-on (10.86\%), 
    \\
    Broadside (6.57\%), 
    Bike/Pedestrian (6.7\%),  
    Hit object (5.81\%)
    ~\cite{learn_crash}
}
\\
\cline{3-3}
% -
& % AV
& \makecell[l]{
    Other (45\%),  
    Rear-end (38\%),    
    Sideswipe (11\%),  
    \\
    Head-on (3\%),
    Hit-object (3\%)
    ~\cite{automated_latent}
} 
\\
\cline{2-3}
% -
& Pedestrian
& \makecell[l]{
    Frontal impact (43.8\%), 
    Side impact (24.1\%),  
    \\
    Car moving forward (23.2\%),
    Back (6.2\%),
    No impact (3.6\%)
    ~\cite{typical_pedestrian}
} 
\\
\cline{2-3}
% -
& \multirow{4}{*}{Bicycle}
& \makecell[l]{
    For bicycle:
    Side (54.7\%),
    Frontal (19.9\%), 
    \\
    Scrape (14.2\%),
    Rear-end (8.2\%), 
    Others (3\%), 
    \\
    For vehicle: 
    Left hood (24.3\%),
    \\
    Frontal hood (17.6\%),
    Right hood (26.7\%),
    \\
    Left back (4.1\%),
    Back (3\%),
    Right back (2.6\%), 
    \\
    Left body (9.7\%),
    Right body (12\%)
    ~\cite{car-bicycle_analysis}
} 
\\
\cline{3-3}
% -
& % Bicycle
& \makecell[l]{
    Front (64.4\%),  
    Right (19.4\%), 
    Left (10.6\%),  
    Rear (5.6\%)
    ~\cite{identifying_factors}
} 
\\
\midrule
%% end Collision Type

%% factor: Speed
\parbox[t]{4pt}{
\multirow{4}{*}{
    \rotatebox[origin=c]{90}{
        \textbf{Speed}
    }
}
}
& \multirow{2}{*}{AV}
& \makecell[l]{
    % speed limit:   
    \textless{}=25mph (88.54\%),  
    \textgreater{}25mph (21.88\%)
    ~\cite{divergent_effect}
} 
\\
\cline{3-3}
% -
& % AV
& \makecell[l]{
    {[}0,15{]} (31.8\%), 
    {[}15,30{]} (17.3\%), 
    {[}30,45{]} (16.2\%),
    \\
    {[}45,60{]} (16.2\%), 
    {[}60.75{]} (15\%), 
    {[}75,90{]} (2.9\%), 
    {[}90,105{]} (0.6\%)
    m/s
    ~\cite{avoid}
} 
\\
\cline{2-3}
% -
& Pedestrian
& \makecell[l]{
    % vehicle speed: 
    2-10m/s (50.8\%),
    10-20m/s (42.9\%), 
    \\
    20-30m/s (5.9\%),
    \textgreater{} 30m/s (0.5\%)
    ~\cite{pedestrian_causation}
} 
\\
\cline{2-3}
% -
& Bicycle
& Speeding (33.1\%)~\cite{car-bicycle_analysis}
\\
\midrule
%% end Speed

%% factor: Weather
\parbox[t]{0pt}{
\multirow{7}{*}{
    \rotatebox[origin=c]{90}{
        \textbf{Weather}
    }
}
}
& \multirow{3}{*}{AV}
& \makecell[l]{
    Clear weather (88.54\%),  
    Cloudy (5.21\%) ,   
    \\
    Raining (3.13\%),  
    Fig/Visibility (2.08\%)
    ~\cite{divergent_effect}
} 
\\
\cline{3-3}
% -
& % AV
& \makecell[l]{
    Clear (77.42\%), 
    Cloudy (19.35\%), 
    % \\
    Raining (12.15\%),
    Fog (1.08\%)
    ~\cite{analysis_poi}
} 
\\
\cline{3-3}
% -
& % AV
& \makecell[l]{
    Clear(48\%),
    Other(44\%),
    % \\
    Cloudy(5\%), 
    Raining(2\%), 
    Fog(1\%)
    ~\cite{automated_latent}
} 
\\
\cline{2-3}
% -
& \multirow{4}{*}{Bicycle}
& \makecell[l]{
    Sunny (70.87\%),
    Rain (15.72\%), 
    Fog (7.11\%),
    \\
    Snow (2.6\%),
    Rain (3.7\%)
    ~\cite{car-bicycle_analysis}
} 
\\
\cline{3-3}
% -
& % Bicycle
& \makecell[l]{
    Clear (68.9\%), 
    Rain/Snow/Fog (16.7\%),  
    Cloudy (14.4\%)
    ~\cite{identifying_factors}
} 
\\
\cline{3-3}
% -
& % Bicycle
& \makecell[l]{
    Visibility fine (82.8\%),
    Visibility reduced (14.9\%), 
    Other (2.3\%)
    ~\cite{single_bicycle_crash}
} 
\\
\midrule
%% end Weather

%% factor: Accident Location
\parbox[t]{0pt}{
\multirow{7}{*}[-20pt]{
    \rotatebox[origin=c]{90}{
        \textbf{Accident Location}
    }
}
}
& \multirow{5}{*}{AV}
& \makecell[l]{
    Road Type:
    Intersection (65.63\%)
    \\
    Street Width:
    \textless{}=60 feet(78.13\%)
    % \\
    Trees: 80.21\% 
    ~\cite{divergent_effect}
} 
\\
\cline{3-3}
% -
& % AV
& \makecell[l]{
    Highway/Freeway (32.0\%), 
    Unknown (37.6\%), 
    Intersection (13.6\%),
    \\
    Street (13.4\%), 
    Rural road (2.2\%),
    % \\
    Parking lot (1.3\%)
    ~\cite{avoid}
} 
\\
\cline{3-3}
% -
& % AV
& \makecell[l]{
    Intersection (47.31\%), 
    Street (35.48\%),  
    \\
    Highway (13.98\%),  
    Parking lot (3.23\%)
    ~\cite{analysis_poi}
}
\\
\cline{3-3}
% -
& % AV
& Intersection (73.5\%)~\cite{exploratory_cal}
\\
\cline{3-3}
% -
& % AV
& \makecell[l]{
    Intersections (69.72\%),    
    Street (21.71\%),     
    Expressway (4.74\%)
    ~\cite{learn_crash}
} 
\\
\cline{2-3}
% -
& \multirow{2}{*}{Bicycle}
& \makecell[l]{
    Road Type:
    Straight road (23.9\%),  
    \\
    Ramp (9.4\%),
    Four-leg intersection (45.6\%),  
    \\
    Three-leg intersection (21.1\%), 
    Single-lane (5.6\%),  
    \\
    Two-lane two-way (7.8\%), 
    Four-lane two-way (24.4\%),  
    \\
    Six-lane, two-way (62.2\%), 
    \\
    Road condition:
    Dry (78.9\%),  
    Wet (16.7\%),
    Water (4.4\%)
    ~\cite{identifying_factors}
} 
\\
\cline{3-3}
% -
& % Bicycle
& \makecell[l]{
    Urban (79\%), 
    Rural (21\%)  
    % \\
    Road condition:
    Dry road surface (31\%),
    \\
    Slippery (49.6\%),
    Wet (18.9\%)
    ~\cite{single_bicycle_crash}
} 
\\
\midrule
%% end Accident Location

%% factor: Vehicle State While Collide.
\parbox[t]{5pt}{
\multirow{6}{*}[-20pt]{
    \rotatebox[origin=c]{90}{
        \textbf{\makecell{Vehicle State}}
    }
}
}
& \multirow{5}{*}[-20pt]{AV}
& \makecell[l]{
    Straight  (87.50\%),
    Turning movement (12.50\%)
    ~\cite{divergent_effect}
} 
\\
\cline{3-3}
% -
& % AV
& \makecell[l]{
    Other (36.63\%),  
    Proceeding straight (20.89\%), 
    Unknown (19.89\%),  
    \\
    Left turn (4.95\%),  
    Changing lanes (4.41\%), 
    \\
    Right turn (1.98\%),  
    Backing (1.89\%)
    ~\cite{avoid}
}   
\\
\cline{3-3}
% -
& % AV
& \makecell[l]{
    Stopped (36.08\%),  
    Proceeding straight (29.9\%),
    Right turn (5.15\%), 
    \\
    Slowing/Stopping (10.31\%),
    Left turn (4.12\%), 
    \\
    Changing lanes (4.12\%),  
    Parking maneuver (2.06\%)
    ~\cite{analysis_poi}
}  
\\
\cline{3-3}
% -
& % AV
& \makecell[l]{
    Left turn (11.5\%),  
    Right turn (21.2\%),
    No turning (66.3\%)
    ~\cite{exploratory_cal}
}  
\\
\cline{3-3}
% -
& % AV
& \makecell[l]{
    Other (44.64\%),  
    Stopped (23.21\%),  
    Straight (15.18\%), 
    \\
    Left turn (3.57\%), 
    Right turn (2.68\%)
    ~\cite{automated_latent}
}  
\\
\cline{2-3}
% -
& Pedestrian
& \makecell[l]{
    Vehicle moving forwards  (99.11\%), 
    Parked or reversing  (0.89\%)
    ~\cite{typical_pedestrian}
} 
\\
\midrule
%% end Vehicle State While Collide.

%% factor: Collide With
\parbox[t]{5pt}{
\multirow{2}{*}{
    \rotatebox[origin=l]{90}{
        \textbf{\makecell{Collide \\ With}}
    }
}
}
& AV
& \makecell[l]{
    Non-motor vehicles or 
    pedestrians involved (18.75\%)
    ~\cite{divergent_effect}
}
\\
\cline{2-3}
& Pedestrian
& \makecell[l]{
    Car/taxi (90.88\%),
    Motorcycle (3.97\%),
    Bus (5.97\%),
    \\
    Light goods vehicle (1.95\%), 
    Other (2.09\%),
    \\
    Pedal cycle (1.48\%),
    Unknown vehicle(0.06\%) 
    ~\cite{typical_pedestrian}
}
\\
\midrule
%% end Collide With

%% factor: # of vehicle 
\parbox[t]{5pt}{
\multirow{3}{*}{
    \rotatebox[origin=l]{90}{
        \textbf{\makecell{\# of \\ Vehicles}}
    }
}
}
& \multirow{3}{*}{AV}
& \makecell[l]{
    2 (87.50\%),
    1 (11.46\%),   
    3 (1.04\%)
    ~\cite{divergent_effect}
} 
\\
\cline{3-3}
% -
& % -
& \makecell[l]{
    2: (90.3\%),  
    1 (8\%),  
    3 (1.8\%)
    ~\cite{exploratory_cal}
} 
\\
\cline{3-3}
% -
& % - 
& \makecell[l]{
    2 (84.16\%),  
    1 (12.87\%), 
    Multi (1.97\%)
    ~\cite{automated_latent}
}
\\
% \midrule
%% end # of vehicle 
%% 
\bottomrule
\end{tabular}
}
\label{tab:design:CrashFactors_all}
\end{table}

\section{Comparison with DriveFuzz in Different Modes}
\label{sec:appdenix:2}

% \listoffigures
%% rq2: DriveFuzz in 
%%
\begin{table}[tp]
\centering
\caption{\S~\ref{sec:appdenix:2}: The number of ICSs identified by DriveFuzz}
\label{tab:eval:drivefuzz-IC}
\resizebox{0.8\columnwidth}{!}{%
\begin{tabular}{c|cccc}
\toprule
\textbf{Mutation Mode} & \textbf{All}  & \textbf{Congestion} & \textbf{Entropy} & \textbf{Instability} 
\\ 
\midrule
Running times & 779 & 884        & 1976    & 893   
\\
Detected ICS  & 12   & 10         & 22      & 0 
\\ 
\bottomrule
\end{tabular}%
}
\end{table}

We also ran DriveFuzz in different modes they offer for 36 hours separately, 
the results are presented in Table~\ref{tab:eval:drivefuzz-IC}. 
DriveFuzz can merely detect a few ICSs within the limited runtime regardless of the mode used.
DriveFuzz tends to spend more time exploring the non-collision space than exploring further possibilities from the collision space.
It also stops immediately after finding an ICS and then initiates a new round of testing using a new seed scenario. 

As a result, DriveFuzz not only misses the opportunity to explore the IC scenario space but also spends more time restarting from a new position in the non-collision scenario space, which is unrelated to the previous round.
Also, the ICSs identified by DriveFuzz, after investing a significant amount of time, exhibit a notable repetition, 
which further highlights the inefficiency of its search strategy.
Comparatively, our incremental search strategy that commences from the collision scenario space has exhibited a discernible superiority.

%%
% \section{Appdneix 3}
% \label{sec:appdenix:3}

% Table~\ref{tab:design:CrashFactors_all}

%%
% \input{tables/tab_CrashFactors_values}

% \newpage 
